# Supplementary material for: Towards a Privacy-Preserving Dispute Resolution Protocol on Ethereum
Source: arXiv:2303.00533 source file (2023-11-24)
Supplement: Supplementary file 1 [file AppendixA.tex]

\begin{Def}
A Succinct Non-interactive ARgument of Knowledge (SNARK) on a circuit $C$ is a triple of algorithms $(\setup, \provex, \verifyx)$ such that:
\begin{itemize}
    \item $\setup(C) \rightarrow (\ppx, \vpx)$, i.e. the setup algorithm takes as input the circuit and outputs some public parameter $\ppx$ for the prover and $\vpx$ for the verifier;
    \item $\provex(\ppx, x, w) \rightarrow \pi$, that is the prove algorithm takes as input the public parameters of the prover $\ppx$, the public statement $x$ and the private witness $w$, and outputs a proof $\pi$ that has to be ``short". Usually, short means $\lenx(\pi) = O_{\lambda}(log|C|)$, where with $|C|$ we denote the number of gates of the circuit, while $\lambda$ is the security parameter;
    \item  $\verifyx(\vpx, x, \pi) \rightarrow 0/1$, that is the verify algorithm takes as input the public parameters of the verifier $\vpx$, the public statement $x$ and the proof $\pi$, and outputs 1 if the proof is correct, 0 otherwise. This algorithm has to be ``fast", which means $\timex(\verifyx) = O_{\lambda}(|x|, log|C|)$, where with $|C|$ we denote the number of gates of the circuit and with $|x|$ we denote the length of the public statement, while $\lambda$ is the security parameter.
\end{itemize}

\end{Def}
This family of algorithms must satisfy the following requirements:
\begin{itemize}
    \item \textit{Completeness}: for each $x,w$ such that $C(x,w)=0$, we have that
    \[\mathbb{P}[\verifyx(\vpx, x, \provex(\ppx, x, w)) = \accept] = 1;\]
    \item \textit{Adaptively Knowledge Soundness}: for every $\pptx$ adversary $\mathcal{A}$ such that
    \[ (\ppx, \vpx) \leftarrow \setup(C), \hskip1cm \pi \leftarrow \mathcal{A}(\ppx, x),\]
    \[ \mathbb{P}[\verifyx(\vpx, x, \pi) = \accept] > \frac{1}{10^6},\]
     (so, it is non-negligible), there is a $\pptx$ extractor $\mathcal{E}$ that uses $\mathcal{A}$ such that
    \[ w \leftarrow \mathcal{E}(C,x), \hskip1cm \mathbb{P}[\verifyx(\vpx, x, \pi) = \accept] > \frac{1}{10^6} - \epsilon,\]
    where $\epsilon$ is a negligible value.
    \item \textit{Statistical Zero-knowledge}: there exists a $\pptx$ algorithm $\mathcal{S}$, called simulator, such that the following two distributions are statistically close:
    \[D_0 = \{ \pi_0 \leftarrow \provex(\ppx,x,w) \,\, | \,\, (\ppx,\vpx) \leftarrow \setup(C) \}, \]
    \[D_1 = \{ \pi_1 \leftarrow \mathcal{S}(\ppx,\vpx,x) \,\, | \,\, (\ppx,\vpx) \leftarrow \setup(C) \}. \]
\end{itemize}

The algorithm used currently by Semaphore and MACI is the Groth16 protocol \cite{groth2016size}. However, there are also other possibilities, for example an algorithm that is showing promise and is already being used by blockchains such as ZCash \cite{miers2013zerocoin} is Halo \cite{bowe2019recursive}, which does not need a trusted setup.
